# Supplementary material for: CXR-LT 2024: A MICCAI challenge on long-tailed, multi-label, and zero-shot disease classification from chest X-ray
Source: arXiv:2506.07984 source file (2025-06-09)
Supplement: Supplementary file 1 [file supplementary_v2.pdf]

## Supplementary Material

# CXR-LT 2024: A MICCAI challenge on long-tailed, multi-label, and zero-shot disease classification from chest X-ray

Supplementary Table 1. Final test phase results of the CXR-LT 2024 competition for Task 1. The table presents the precision of the top-4 teams' final models for each of the 40 classes evaluated on the test set.

| Disease | zguo | Tianjie_dai | XYPB | dongkyunk |
|---|---|---|---|---|
| Atelectasis | 0.626 | 0.630 | 0.627 | 0.628 |
| Cardiomegaly | 0.669 | 0.683 | 0.678 | 0.675 |
| Consolidation | 0.250 | 0.259 | 0.253 | 0.251 |
| Edema | 0.551 | 0.551 | 0.553 | 0.547 |
| Enlarged Cardiomediastinum | 0.189 | 0.196 | 0.192 | 0.188 |
| Fracture | 0.380 | 0.364 | 0.328 | 0.367 |
| Lung Lesion | 0.068 | 0.069 | 0.067 | 0.062 |
| Lung Opacity | 0.628 | 0.627 | 0.629 | 0.633 |
| Pleural Effusion | 0.845 | 0.845 | 0.843 | 0.842 |
| Pneumonia | 0.335 | 0.336 | 0.342 | 0.339 |
| Pneumothorax | 0.608 | 0.597 | 0.597 | 0.618 |
| Support Devices | 0.927 | 0.925 | 0.927 | 0.926 |
| Granuloma | 0.317 | 0.269 | 0.296 | 0.342 |
| Normal | 0.331 | 0.333 | 0.335 | 0.334 |
| Calcification of the Aorta | 0.172 | 0.163 | 0.164 | 0.173 |
| Emphysema | 0.263 | 0.262 | 0.258 | 0.274 |
| Fibrosis | 0.169 | 0.167 | 0.169 | 0.138 |
| Hernia | 0.572 | 0.583 | 0.580 | 0.550 |
| Infiltration | 0.064 | 0.064 | 0.067 | 0.064 |
| Mass | 0.251 | 0.287 | 0.250 | 0.258 |
| Nodule | 0.246 | 0.233 | 0.232 | 0.254 |
| Pleural Thickening | 0.153 | 0.146 | 0.138 | 0.137 |
| Pneumomediastinum | 0.307 | 0.340 | 0.338 | 0.300 |
| Pneumoperitoneum | 0.299 | 0.299 | 0.351 | 0.286 |
| Subcutaneous Emphysema | 0.613 | 0.604 | 0.580 | 0.609 |
| Tortuous Aorta | 0.067 | 0.068 | 0.070 | 0.072 |
| Adenopathy | 0.103 | 0.136 | 0.129 | 0.112 |
| Azygos Lobe | 0.156 | 0.133 | 0.117 | 0.146 |
| Clavicle Fracture | 0.040 | 0.013 | 0.006 | 0.003 |
| Fissure | 0.223 | 0.198 | 0.174 | 0.197 |
| Hydropneumothorax | 0.179 | 0.185 | 0.173 | 0.142 |
| Infarction | 0.011 | 0.008 | 0.011 | 0.011 |
| Kyphosis | 0.086 | 0.086 | 0.107 | 0.073 |
| Lobar Atelectasis | 0.008 | 0.004 | 0.005 | 0.004 |
| Pleural Other | 0.077 | 0.066 | 0.067 | 0.071 |
| Pulmonary Embolism | 0.012 | 0.013 | 0.013 | 0.012 |
| Pulmonary Hypertension | 0.032 | 0.047 | 0.049 | 0.035 |
| Rib Fracture | 0.284 | 0.269 | 0.256 | 0.289 |
| Round(ed) Atelectasis | 0.053 | 0.028 | 0.057 | 0.041 |
| Tuberculosis | 0.062 | 0.060 | 0.073 | 0.064 |
| Mean | 0.281 | 0.279 | 0.277 | 0.277 |

Supplementary Table 2. Final test phase results of the CXR-LT 2024 competition for Task 1. The table presents the F1 of the top-4 teams' final models for each of the 40 classes evaluated on the test set.

| Disease | zguo | Tianjie_dai | XYPB | dongkyunk |
|---|---|---|---|---|
| Atelectasis | 0.566 | 0.549 | 0.557 | 0.556 |
| Cardiomegaly | 0.541 | 0.517 | 0.543 | 0.543 |
| Consolidation | 0.259 | 0.275 | 0.275 | 0.275 |
| Edema | 0.453 | 0.440 | 0.468 | 0.455 |
| Enlarged Cardiomediastinum | 0.232 | 0.220 | 0.229 | 0.229 |
| Fracture | 0.347 | 0.320 | 0.359 | 0.324 |
| Lung Lesion | 0.136 | 0.156 | 0.139 | 0.117 |
| Lung Opacity | 0.560 | 0.550 | 0.565 | 0.574 |
| Pleural Effusion | 0.707 | 0.682 | 0.704 | 0.708 |
| Pneumonia | 0.346 | 0.338 | 0.347 | 0.347 |
| Pneumothorax | 0.491 | 0.500 | 0.493 | 0.477 |
| Support Devices | 0.841 | 0.813 | 0.841 | 0.845 |
| Granuloma | 0.346 | 0.347 | 0.393 | 0.358 |
| Normal | 0.360 | 0.359 | 0.379 | 0.373 |
| Calcification of the Aorta | 0.258 | 0.214 | 0.254 | 0.224 |
| Emphysema | 0.293 | 0.313 | 0.314 | 0.283 |
| Fibrosis | 0.245 | 0.255 | 0.244 | 0.225 |
| Hernia | 0.522 | 0.498 | 0.566 | 0.438 |
| Infiltration | 0.114 | 0.109 | 0.119 | 0.109 |
| Mass | 0.263 | 0.299 | 0.300 | 0.263 |
| Nodule | 0.260 | 0.228 | 0.259 | 0.242 |
| Pleural Thickening | 0.202 | 0.208 | 0.209 | 0.177 |
| Pneumomediastinum | 0.370 | 0.392 | 0.407 | 0.391 |
| Pneumoperitoneum | 0.444 | 0.443 | 0.481 | 0.386 |
| Subcutaneous Emphysema | 0.593 | 0.572 | 0.605 | 0.564 |
| Tortuous Aorta | 0.113 | 0.133 | 0.125 | 0.126 |
| Adenopathy | 0.151 | 0.156 | 0.172 | 0.146 |
| Azygos Lobe | 0.163 | 0.326 | 0.221 | 0.289 |
| Clavicle Fracture | 0.065 | 0.000 | 0.000 | 0.000 |
| Fissure | 0.257 | 0.230 | 0.247 | 0.217 |
| Hydropneumothorax | 0.313 | 0.270 | 0.258 | 0.231 |
| Infarction | 0.000 | 0.000 | 0.025 | 0.017 |
| Kyphosis | 0.167 | 0.123 | 0.125 | 0.129 |
| Lobar Atelectasis | 0.000 | 0.000 | 0.000 | 0.000 |
| Pleural Other | 0.117 | 0.121 | 0.125 | 0.152 |
| Pulmonary Embolism | 0.000 | 0.000 | 0.006 | 0.015 |
| Pulmonary Hypertension | 0.011 | 0.062 | 0.099 | 0.079 |
| Rib Fracture | 0.326 | 0.287 | 0.313 | 0.293 |
| Round(ed) Atelectasis | 0.000 | 0.000 | 0.043 | 0.081 |
| Tuberculosis | 0.143 | 0.136 | 0.162 | 0.151 |
| Macro F1 | 0.289 | 0.286 | 0.299 | 0.285 |
| Micro F1 | 0.471 | 0.455 | 0.474 | 0.462 |

Supplementary Table 3. Final test phase results of the CXR-LT 2024 competition for Task 1. The table presents the False Negative Rate (FNR) of the top-4 teams' final models for each of the 40 classes evaluated on the test set.

| Disease | zguo | Tianjie_dai | XYPB | dongkyunk |
|---|---|---|---|---|
| Atelectasis | 0.069 | 0.052 | 0.059 | 0.556 |
| Cardiomegaly | 0.064 | 0.036 | 0.063 | 0.543 |
| Consolidation | 0.271 | 0.305 | 0.307 | 0.275 |
| Edema | 0.121 | 0.108 | 0.131 | 0.455 |
| Enlarged Cardiomediastinum | 0.168 | 0.083 | 0.139 | 0.229 |
| Fracture | 0.362 | 0.394 | 0.438 | 0.324 |
| Lung Lesion | 0.851 | 0.814 | 0.761 | 0.117 |
| Lung Opacity | 0.042 | 0.033 | 0.045 | 0.574 |
| Pleural Effusion | 0.061 | 0.048 | 0.059 | 0.708 |
| Pneumonia | 0.050 | 0.024 | 0.049 | 0.347 |
| Pneumothorax | 0.264 | 0.277 | 0.263 | 0.477 |
| Support Devices | 0.055 | 0.049 | 0.056 | 0.845 |
| Granuloma | 0.529 | 0.614 | 0.596 | 0.358 |
| Normal | 0.101 | 0.101 | 0.130 | 0.373 |
| Calcification of the Aorta | 0.468 | 0.331 | 0.420 | 0.224 |
| Emphysema | 0.440 | 0.467 | 0.472 | 0.283 |
| Fibrosis | 0.509 | 0.512 | 0.545 | 0.225 |
| Hernia | 0.379 | 0.329 | 0.378 | 0.438 |
| Infiltration | 0.802 | 0.854 | 0.768 | 0.109 |
| Mass | 0.560 | 0.530 | 0.621 | 0.263 |
| Nodule | 0.568 | 0.474 | 0.571 | 0.242 |
| Pleural Thickening | 0.554 | 0.557 | 0.679 | 0.177 |
| Pneumomediastinum | 0.497 | 0.527 | 0.510 | 0.391 |
| Pneumoperitoneum | 0.597 | 0.551 | 0.473 | 0.386 |
| Subcutaneous Emphysema | 0.109 | 0.087 | 0.127 | 0.564 |
| Tortuous Aorta | 0.836 | 0.713 | 0.784 | 0.126 |
| Adenopathy | 0.819 | 0.675 | 0.748 | 0.146 |
| Azygos Lobe | 0.849 | 0.472 | 0.660 | 0.289 |
| Clavicle Fracture | 0.958 | 1.000 | 1.000 | 0.000 |
| Fissure | 0.541 | 0.519 | 0.645 | 0.217 |
| Hydropneumothorax | 0.636 | 0.594 | 0.693 | 0.231 |
| Infarction | 1.000 | 1.000 | 0.986 | 0.017 |
| Kyphosis | 0.703 | 0.533 | 0.713 | 0.129 |
| Lobar Atelectasis | 1.000 | 1.000 | 1.000 | 0.000 |
| Pleural Other | 0.913 | 0.889 | 0.858 | 0.152 |
| Pulmonary Embolism | 1.000 | 1.000 | 0.996 | 0.015 |
| Pulmonary Hypertension | 0.994 | 0.958 | 0.891 | 0.079 |
| Rib Fracture | 0.499 | 0.517 | 0.526 | 0.293 |
| Round(ed) Atelectasis | 1.000 | 1.000 | 0.971 | 0.081 |
| Tuberculosis | 0.759 | 0.756 | 0.665 | 0.151 |
| Macro FNR | 0.525 | 0.495 | 0.520 | 0.466 |
| Micro FNR | 0.151 | 0.135 | 0.153 | 0.142 |

Supplementary Table 4. Final test phase results of the CXR-LT 2024 competition for Task 2. The table presents the precision of the top-4 teams' final models for each of the 26 classes evaluated on the golden standard test set.

| Disease | XYPB | zguo | yangz16 | YYama |
|---|---|---|---|---|
| Atelectasis | 0.464 | 0.457 | 0.454 | 0.465 |
| Calcification of the Aorta | 0.680 | 0.643 | 0.566 | 0.633 |
| Cardiomegaly | 0.747 | 0.711 | 0.717 | 0.739 |
| Consolidation | 0.466 | 0.437 | 0.450 | 0.466 |
| Edema | 0.537 | 0.582 | 0.564 | 0.585 |
| Emphysema | 0.364 | 0.386 | 0.379 | 0.335 |
| Enlarged Cardiomediastinum | 0.347 | 0.346 | 0.348 | 0.339 |
| Fibrosis | 0.549 | 0.456 | 0.543 | 0.536 |
| Fracture | 0.538 | 0.622 | 0.619 | 0.492 |
| Hernia | 0.789 | 0.748 | 0.840 | 0.741 |
| Infiltration | 0.052 | 0.049 | 0.056 | 0.045 |
| Lung Lesion | 0.037 | 0.048 | 0.055 | 0.042 |
| Lung Opacity | 0.657 | 0.658 | 0.642 | 0.662 |
| Mass | 0.430 | 0.388 | 0.384 | 0.401 |
| Normal | 0.726 | 0.795 | 0.741 | 0.727 |
| Nodule | 0.326 | 0.430 | 0.335 | 0.376 |
| Pleural Effusion | 0.837 | 0.850 | 0.842 | 0.835 |
| Pleural Other | 0.339 | 0.262 | 0.259 | 0.307 |
| Pleural Thickening | 0.333 | 0.321 | 0.372 | 0.258 |
| Pneumomediastinum | 0.832 | 0.791 | 0.768 | 0.823 |
| Pneumonia | 0.127 | 0.165 | 0.125 | 0.149 |
| Pneumoperitoneum | 0.732 | 0.605 | 0.641 | 0.581 |
| Pneumothorax | 0.665 | 0.657 | 0.630 | 0.639 |
| Subcutaneous Emphysema | 0.849 | 0.802 | 0.760 | 0.783 |
| Support Devices: 0.9643 | 0.964 | 0.961 | 0.944 | 0.958 |
| Tortuous Aorta | 0.302 | 0.319 | 0.245 | 0.317 |
| Mean | 0.527 | 0.519 | 0.511 | 0.509 |

Supplementary Table 5. Final test phase results of the CXR-LT 2024 competition for Task 2. The table presents the F1 of the top-4 teams' final models for each of the 26 classes evaluated on the golden standard test set.

| Disease | XYPB | zguo | yangz16 | YYama |
|---|---|---|---|---|
| Atelectasis | 0.517 | 0.522 | 0.486 | 0.523 |
| Calcification of the Aorta | 0.628 | 0.543 | 0.000 | 0.548 |
| Cardiomegaly | 0.618 | 0.625 | 0.603 | 0.619 |
| Consolidation | 0.439 | 0.432 | 0.053 | 0.432 |
| Edema | 0.547 | 0.530 | 0.413 | 0.545 |
| Emphysema | 0.321 | 0.414 | 0.000 | 0.274 |
| Enlarged Cardiomediastinum | 0.437 | 0.415 | 0.032 | 0.433 |
| Fibrosis | 0.546 | 0.455 | 0.000 | 0.526 |
| Fracture | 0.552 | 0.583 | 0.154 | 0.544 |
| Hernia | 0.737 | 0.684 | 0.690 | 0.743 |
| Infiltration | 0.094 | 0.042 | 0.000 | 0.000 |
| Lung Lesion | 0.048 | 0.000 | 0.000 | 0.000 |
| Lung Opacity | 0.684 | 0.685 | 0.625 | 0.685 |
| Mass | 0.426 | 0.358 | 0.261 | 0.415 |
| Normal | 0.737 | 0.673 | 0.053 | 0.646 |
| Nodule | 0.364 | 0.375 | 0.000 | 0.310 |
| Pleural Effusion | 0.714 | 0.721 | 0.745 | 0.714 |
| Pleural Other | 0.240 | 0.000 | 0.000 | 0.095 |
| Pleural Thickening | 0.383 | 0.339 | 0.000 | 0.391 |
| Pneumomediastinum | 0.767 | 0.789 | 0.326 | 0.776 |
| Pneumonia | 0.114 | 0.112 | 0.000 | 0.118 |
| Pneumoperitoneum | 0.681 | 0.579 | 0.222 | 0.585 |
| Pneumothorax | 0.513 | 0.545 | 0.619 | 0.539 |
| Subcutaneous Emphysema | 0.808 | 0.808 | 0.720 | 0.842 |
| Support Devices: 0.9643 | 0.877 | 0.875 | 0.884 | 0.873 |
| Tortuous Aorta | 0.174 | 0.150 | 0.000 | 0.143 |
| Macro F1 | 0.499 | 0.471 | 0.260 | 0.474 |
| Micro F1 | 0.564 | 0.562 | 0.530 | 0.562 |

Supplementary Table 6. Final test phase results of the CXR-LT 2024 competition for Task 2. The table presents the False Negative Rate (FNR) of the top-4 teams' final models for each of the 26 classes evaluated on the golden standard test set.

| Disease | XYPB | zguo | yangz16 | YYama |
|---|---|---|---|---|
| Atelectasis | 0.016 | 0.032 | 0.456 | 0.016 |
| Calcification of the Aorta | 0.426 | 0.532 | 1.000 | 0.511 |
| Cardiomegaly | 0.019 | 0.025 | 0.484 | 0.025 |
| Consolidation | 0.176 | 0.189 | 0.973 | 0.203 |
| Edema | 0.040 | 0.040 | 0.683 | 0.040 |
| Emphysema | 0.552 | 0.379 | 1.000 | 0.655 |
| Enlarged Cardiomediastinum | 0.246 | 0.297 | 0.983 | 0.229 |
| Fibrosis | 0.455 | 0.545 | 1.000 | 0.545 |
| Fracture | 0.229 | 0.229 | 0.917 | 0.292 |
| Hernia | 0.263 | 0.316 | 0.474 | 0.316 |
| Infiltration | 0.750 | 0.917 | 1.000 | 1.000 |
| Lung Lesion | 0.833 | 1.000 | 1.000 | 1.000 |
| Lung Opacity | 0.010 | 0.010 | 0.367 | 0.015 |
| Mass | 0.350 | 0.400 | 0.850 | 0.450 |
| Normal | 0.054 | 0.081 | 0.973 | 0.135 |
| Nodule | 0.636 | 0.636 | 1.000 | 0.667 |
| Pleural Effusion | 0.011 | 0.005 | 0.240 | 0.005 |
| Pleural Other | 0.842 | 1.000 | 1.000 | 0.947 |
| Pleural Thickening | 0.591 | 0.545 | 1.000 | 0.591 |
| Pneumomediastinum | 0.200 | 0.200 | 0.800 | 0.257 |
| Pneumonia | 0.182 | 0.182 | 1.000 | 0.136 |
| Pneumoperitoneum | 0.333 | 0.542 | 0.875 | 0.500 |
| Pneumothorax | 0.020 | 0.082 | 0.388 | 0.020 |
| Subcutaneous Emphysema | 0.048 | 0.048 | 0.357 | 0.048 |
| Support Devices: 0.9643 | 0.045 | 0.050 | 0.122 | 0.050 |
| Tortuous Aorta | 0.879 | 0.909 | 1.000 | 0.909 |
| Macro FNR | 0.316 | 0.365 | 0.767 | 0.368 |
| Micro FNR | 0.148 | 0.165 | 0.570 | 0.167 |

Supplementary Table 7. Final test phase results of the CXR-LT 2024 competition for Task 3. The table presents the precision of the top-3 teams' final models for each of the 5 classes evaluated on the test set.

| Disease | yyge | zhangRuichi | pamessina |
|---|---|---|---|
| Bulla | 0.013 | 0.011 | 0.038 |
| Cardiomyopathy | 0.036 | 0.007 | 0.065 |
| Hilum | 0.359 | 0.389 | 0.252 |
| Osteopenia | 0.034 | 0.037 | 0.036 |
| Scoliosis | 0.205 | 0.158 | 0.036 |
| Mean | 0.129 | 0.116 | 0.110 |

Supplementary Table 8. Final test phase results of the CXR-LT 2024 competition for Task 3. The table presents the F1 of the top-3 teams' final models for each of the 5 classes evaluated on the test set.

| Disease | yyge | zhangRuichi | pamessina |
|---|---|---|---|
| Bulla | 0.000 | 0.000 | 0.028 |
| Cardiomyopathy | 0.062 | 0.000 | 0.026 |
| Hilum | 0.000 | 0.000 | 0.289 |
| Osteopenia | 0.061 | 0.000 | 0.019 |
| Scoliosis | 0.252 | 0.176 | 0.107 |
| Macro F1 | 0.075 | 0.035 | 0.094 |
| Micro F1 | 0.047 | 0.022 | 0.182 |

Supplementary Table 9. Final test phase results of the CXR-LT 2024 competition for Task 3. The table presents the False Negative Rate (FNR) of the top-3 teams' final models for each of the 5 classes evaluated on the test set.

| Disease | yyge | zhangRuichi | pamessina |
|---|---|---|---|
| Bulla | 1.000 | 1.000 | 0.260 |
| Cardiomyopathy | 0.958 | 1.000 | 0.231 |
| Hilum | 1.000 | 1.000 | 0.584 |
| Osteopenia | 0.892 | 1.000 | 0.308 |
| Scoliosis | 0.762 | 0.896 | 0.616 |
| Macro FNR | 0.923 | 0.979 | 0.400 |
| Micro FNR | 0.974 | 0.989 | 0.580 |
